# Supplementary material for: First-Principles Prediction of Electronic Transport in Experimental Semiconductor Heterostructures via Physics-Based Machine Learning
Source: arXiv:2011.08426 source file (2020-11-17)
Supplement: Supplementary file 1 [file supplementary.pdf]

# First-Principles Prediction of Electronic Transport in Experimental Semiconductor Heterostructures via Physics-Based Machine Learning–Supplementary Information

Artem K Pimachev[1] and Sanghamitra Neogi[1,*]

[1]*Ann and H.J. Smead Aerospace Engineering Sciences, University of Colorado Boulder, Boulder, Colorado 80303, USA*

(Dated: November 16, 2020)

## DESCRIPTION OF FINGERPRINTING FEATURES

In this section we describe the various geometrical and physical features we used to train the ML model. Our choice of features and their functional forms closely follow the feature categories implemented by Ward et al. [1], with slight modifications, as we discuss below. In total, our method describes each configuration by 100 features of the following categories.

### Global Structural Features

We include a set of global structural features based on the lattice parameters and compositions of the structures. We compute the effective lattice constant features $a$, $b$, and $c$ by dividing the Si/Ge structure dimensions ($L_x$, $L_y$, $L_z$) with the number of conventional cells of which the corresponding dimension is comprised of ($N_x$, $N_y$, $N_z$), respectively. The atomic composition of Si and Ge in a given structure is also included as a global atomic feature, calculated from the fraction of atoms of a given type present in the structure. In total, a given configuration is described by four global features $a$, $b$, $c$, and Ge concentration. We could have chosen Si concentration in the configurations as well, since in these binary systems they are complementary of each other. In total, our method describes each configuration by four global physical features.

### Local Features

The main idea in our approach is to represent the crystal structure by a crystal graph that encodes both atomic information and bonding environment between atoms, and then use the graph to extract features that are optimum for predicting electronic transport properties by training with DFT calculated data. In Fig. 2 of the main manuscript, we show a crystal graph $G$, defined by nodes representing atoms and edges representing connections between atoms in a structure. The crystal graph allows multiple edges between the same pair of end nodes. Each node $i$ is represented by a feature vector $\mathbf{v}_i$, encoding the property of the atom corresponding to node $i$: $\mathbf{v}_i :=$ [elemental-property, structural factors {effective coordination number, maximum packing efficiency, environment heterogeneity, local ordering ($Q$)}]. Below, we provide details of the features.

### Elemental-Property Features

These features are based on the difference in atomic elemental properties between a central atom and its neighbors. The local property difference for each atom is defined as the Voronoi face area weighted mean of the absolute difference in the elemental property between a central atom and each of its neighbors:

$$\delta_p = \frac{\sum_n A_n * |p_n - p_i|}{\sum_n A_n}, \quad (1)$$

where $\delta_p$ is the local property difference for a elemental property $p$, $p_i$ is the elemental property of the central atom, $p_n$ is the elemental property of neighboring atom $n$, and $A_n$ is the area of the face adjacent to neighbor $n$.

We compute the mean, mean absolute deviation, maximum, and minimum of the distribution of local elemental property difference in a configuration, to compute the local elemental-property features. Our models contain only two atom types in the configurations (Si and Ge). Therefore, the elemental properties vary only slightly in the configurations, yielding a small variation in the local element property features values. For example, the approximate absolute difference between the electronegativity of each Si atom surrounded by its neighbors is therefore $|1.90 - 2.01| = 0.11$ (the difference between Si (1.90) and Ge (2.01)), and the variation of this value across the configuration is almost negligible. We consider only one elemental-property based feature, computed from the difference in electronegativities of the atoms. In total, our method describes each configuration by four local elemental-property based features.

### Effective Coordination Number

As in Ref. [1], we define the effective coordination number of an atom $X$ by a function of the face areas of its Voronoi polyhedron:

$$CN_{eff} = \frac{(\sum_n A_n)^2}{\sum_n A_n^2}, \quad (2)$$

where $A_n$ is the area of face $n$ of a single Voronoi cell in the tessellation, enclosing the volume around atom $X$. Figure 1 shows a schematic Voronoi Cell in the interface region of a representative binary heterostructure. We describe each configuration by four effective coordination number features. We compute the maximum, minimum, mean, and mean absolute deviation (MAD) in effective coordination numbers over all the atoms in a given configuration, and consider them as features. The mean absolute deviation ($\hat{f}$) of a quantity ($f$) is defined as

$$\hat{f} = \frac{1}{N}\sum_i |f_i - \bar{f}|, \quad (3)$$

where $f_i$ is the value of the $i^{\text{th}}$ sample, $N$ is the number of samples, and $\bar{f}$ is the mean.

## Maximum Packing Efficiency

To estimate the maximum packing efficiency for each atom, we divide the volume of the largest sphere centered on the atom that can be placed inside its Voronoi cell, by the volume of the cell. The mean, mean absolute deviation, maximum, and minimum of the distribution of maximum packing efficiency in a configuration are used as the features. In total, our method describes each configuration by four maximum packing efficiency features.

## Environment Heterogeneity Features

These features are designed to measure the variation in the local bonding environments due to strain in the structures.

### *Effective Bond Length*

We define the effective bond length of an atom $i$, $\bar{l}_i$, as the Voronoi-face-area-weighted average of the absolute distance between the atom and each of its neighbors,

$$\bar{l}_i = \frac{\sum_n A_n * ||\vec{r_n} - \vec{r_i}||_2}{\sum_n A_n}, \quad (4)$$

where $\vec{r_i}$ is its position, and $A_n$ and $\vec{r_n}$ are the face area and the position of the $n^{th}$ neighbor, respectively. We describe each configuration by four effective bond length features: the maximum, the minimum, the mean, and the mean absolute deviation of effective bond lengths among all the atoms in a given configuration.

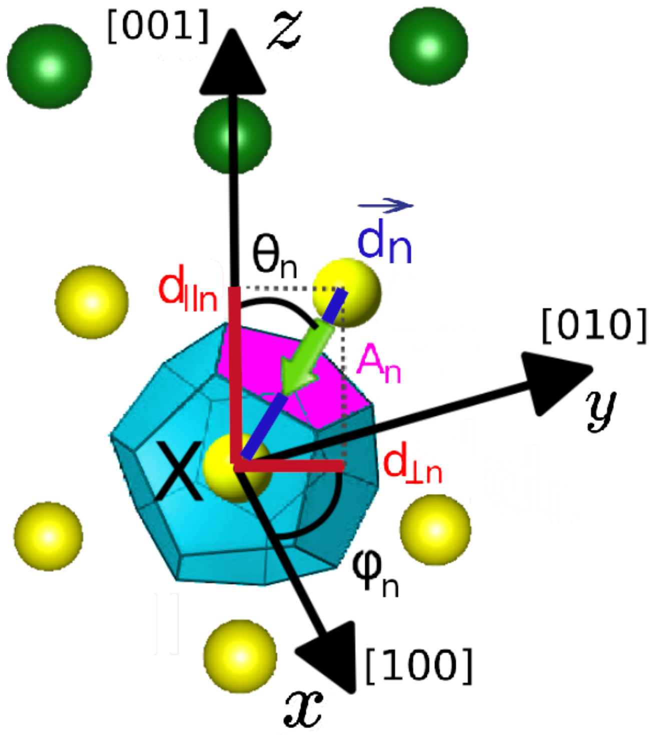


FIG. 1. Schematic representation of a Voronoi cell in a representative binary heterostructure. The heterogeneous regions are stacked along the [001] direction. The green arrow shows a step along a path connecting atom X with neighboring atoms within a crystal graph representation. The step traverses the Voronoi cell face with area $A_n$ (magenta). The length of the step is equal to the interatomic distance $d_n$. $\vec{d_n}$ makes an angle $\theta$ with the $z$ direction, along the SL growth direction, and the projection of $\vec{d_n}$ in the $x-y$ plane makes an angle $\phi$ with the $x$ direction. The component of $\vec{d_n}$ parallel to [001] and the projection of $\vec{d_n}$ in the $x-y$ plane are shown as $d_{||n}$ and $d_{\perp n}$, respectively.

### *Bond Length Variance*

The bond length variance reflects the distribution in bond lengths between each neighbor of an atom, and is computed by:

$$\hat{l}_i = \frac{\sum_n |A_n * ||\vec{r_n} - \vec{r_i}||_2 - \bar{l}_i|}{\bar{l}_i \sum_n A_n}, \quad (5)$$

with the symbols representing quantities as described above. Unlike Ref. 1, we do not normalize these features in order to capture the variation in the effective bond length due to changes in the strain environments. Our method describes each configuration by four effective bond length variance features: the maximum, the minimum, the mean, and the mean absolute deviation of bond length variance values.

*Voronoi Cell Volume*

We construct a Voronoi cell volume segment as a polyhedron with the central atom as a vertex and one of its surface faces as a base. For example, we can construct 12 such volume segments for each atom in a perfect FCC lattice, since each atom has 12 neighbors and 12 faces in the Wigner-Seitz cell in the lattice. We compute the total, the smallest, the largest, the mean volume and the mean absolute deviation of the volumes of each atom's Voronoi cell volume segments. We compute the maximum, the minimum, the mean, and the deviation of each of these five atomic features among all the atoms in a given configuration. We describe each configuration by $5 \times 4 = 20$ Voronoi cell volume features. These features are not normalized so that the the ML model is trained on the strain-induced changes in the Voronoi cell volumes.

*Voronoi Cell Surface Area*

In addition, we compute the different statistical parameters of the surface areas of each atom's Voronoi cell segments: the total, the smallest, the largest, the mean surface area, and the mean absolute deviation. We determine the maximum, the minimum, the mean, and the deviation values of the Voronoi cell surface areas in a given configuration. In total, our method describes each configuration by $5 \times 4 = 20$ Voronoi cell surface area features. These features are also not normalized in order to train the ML model on strain-induced changes in the Voronoi cell surface areas.

**Local Ordering Features**

We construct the ordering features adopting a slightly modified form of the Warren-Cowley order parameters. These parameters measure the structural order of the environment; to what extent the atomic arrangement in a crystal structure is different from purely-random distributions [2]. Below, we illustrate the procedure to determine the order parameters using the example of a simple lattice. To compute the order parameters, we express the crystal structures by crystal graphs connecting the neighboring atoms, that encodes both atomic information and bonding environment between atoms [3–5]. Figure 2(a) shows a representative crystal graph of a simpler two-dimensional Voronoi lattice. We choose to discuss the simpler arrangement since the complexity of a crystal graph representing a higher dimensional crystal structure will be harder to visualize and therefore, demonstrate the concept. To construct the crystal graphs, we determine all possible paths originating from neighboring atoms and ending on a given atom $X$ in the structure. Figure 2(a) shows the different paths connecting atom at position

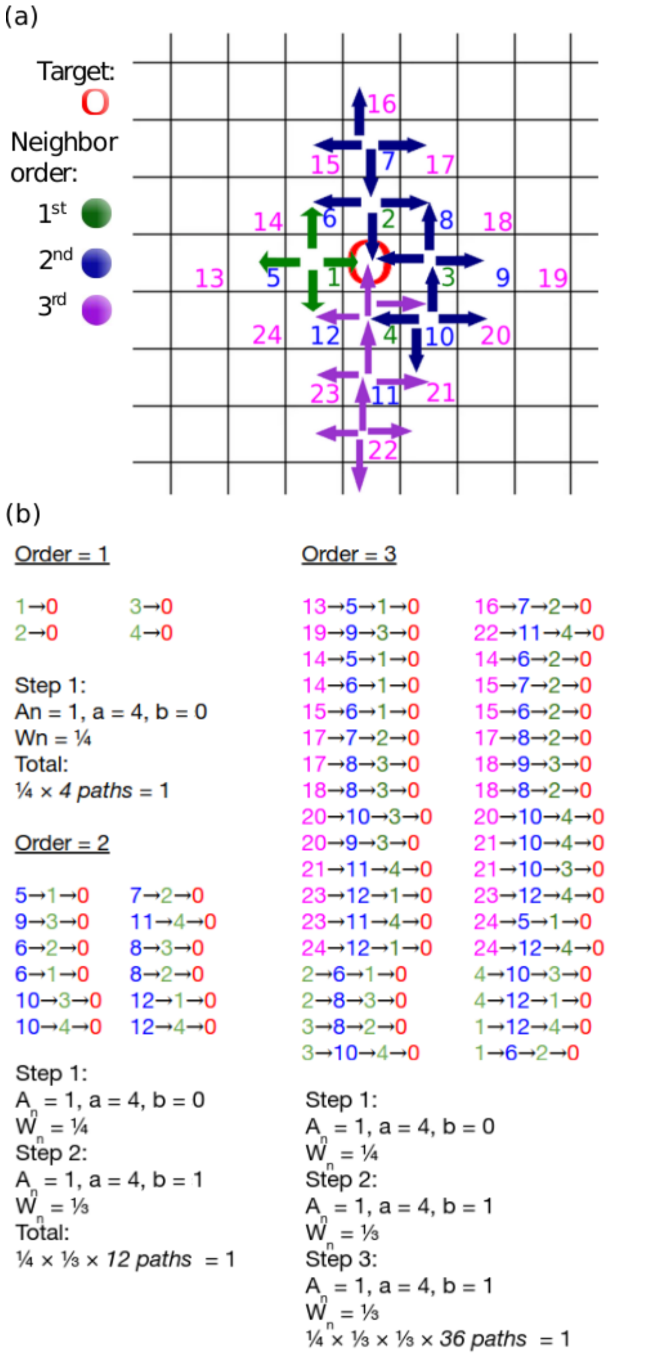


FIG. 2. (a) Example of a 2D graph of a square Voronoi lattice. Green, blue, and purple arrows depict paths of lengths 1, 2, and 3, respectively. 0 represents the end of each path. Only non-backtracking steps are shown with the arrows. Example of path of length 1: $1 \to 0$; Examples of paths of length 2: $10 \to 3 \to 0$ and $7 \to 2 \to 0$; Example of length-3-path: $22 \to 11 \to 4 \to 0$. (b) Example calculation of the weights for each path shown in (a) and the sum over the effective weights for atom 0.

'0' (representing atom $X$) with neighboring atoms. We consider the paths that include neighboring atoms up to order $= 3$ mostly due to the fact that the computational expense to determine all possible path combinations increases proportionally with the volume of the sphere containing the neighboring atoms, $\sim$order$^3$. The numbers in Fig. 2(a) are used to represent indices of the nearest neighbors of atom '0' of the first (green), second (blue), and third (purple) order. These numbers are used only to tag the atoms, and not used directly in the calculation of the features. Therefore, any numbers or symbols would work as long as they are all different, and can simply express the paths originating from a neighbor to a target.

We only consider the non-backtracking paths connecting neighboring atoms up to order $= 3$ to determine the ordering features. Each step of these selected paths are assigned with a fractional weight, $W_n$, where $n$ is the index of the face of the Voronoi cell the step intersects. $W_n$ is determined from the ratio between the area of the face being crossed ($A_n$), normal to the direction of the step, and the sum over all the face areas the step could possibly cross, that are part of other non-backtracking paths:

$$W_n = \frac{A_n}{\sum_a A_a - \sum_b A_b}. \tag{6}$$

Here the two sums in the denominator are over the face areas that intersect all allowed ($a$) (including $A_n$) and back-tracking ($b$) steps, respectively. The effective weight of a path is determined by multiplying the fractional weight of each steps. The weight of each path can be understood as the probability of taking a certain path, given the probability of taking each step is proportional to the ratio between the area of the face of the Voronoi cell being crossed and the sum over all possible areas. This results in the sum over the effective weights of all possible paths in a given order crystal graph being equal to 1:

$$\sum_{paths} \prod_{steps}^{order} W_n = \sum_{paths} \prod_{steps}^{order} \frac{A_n}{\sum_a A_a - \sum_b A_b} = 1. \tag{7}$$

If the total number of atoms in a configuration is $N$, then we have

$$\sum_X Q_X = \sum_X \sum_{paths} \prod_{steps}^{order} W_n = N \tag{8}$$

Figure 2(b) shows an example calculation of the effective weights, and justification supporting Eq. 7. For the example shown in Fig. 2(a), we obtain 4 paths connecting atom '0' with order $= 1$ neighbors, each with weight $W_n = 1/4$. There are 12 two-step paths each with weight $W_n = 1/4 \times 1/3$ connecting with order $= 2$ neighbors. And there are 36 paths for order $= 3$ neighbors, each

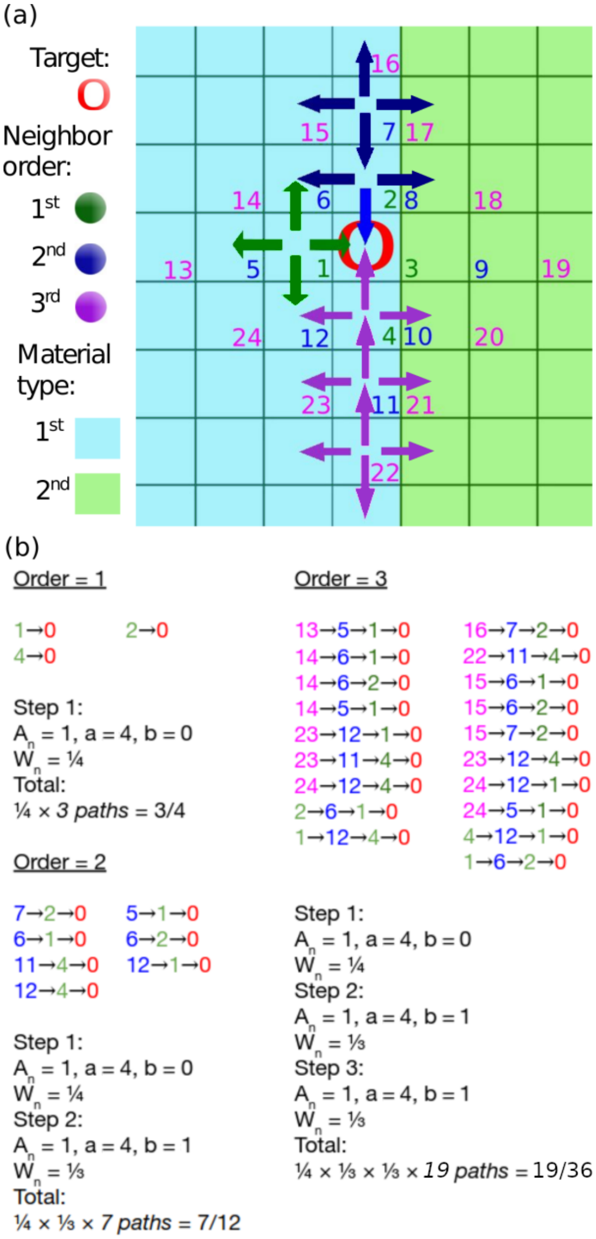


FIG. 3. (a) Example of a 2D graph of a square Voronoi lattice. The lattice configuration shows an interface between two types of materials 1 and 2, shown with a light green and light blue colors, respectively. The paths are constructed ending at the target atom 0, of material type 1. Only paths connecting other type 1 atoms to atom 0 are selected, to determine species-aware order parameters. Green, blue, and purple arrows represent paths of lengths 1, 2, and 3, respectively. Only non-backtracking steps are shown with the arrows. Example of path of length 1: $1 \to 0$; example of paths of length 2: $7 \to 2 \to 0$; example of length-3-path: $22 \to 11 \to 4 \to 0$. (b) The calculation of the weight for each path and the total order parameter for atom 0.

with weight $W_n = 1/4 \times 1/3 \times 1/3$. The sum over the effective path weights for any given order is equal to 1.

We further define a species-aware order parameter for atom $X$ as follows:

$$Q_X^{order} = \sum_{paths} \prod_{steps}^{order} \frac{A_n \delta_{nX}}{\sum_a A_a - \sum_b A_b}. \tag{9}$$

The Kronecker delta function in the numerator restricts consideration of paths connecting only atoms of same type as $X$. To demonstrate the concept of the species-aware order parameters, we show in Figure 3 an illustrative example of a graph connecting atom at position '0' (representing $X$) with neighboring atoms, within a square Voronoi lattice of a system consisting of two materials forming an interface. Figure 3(b) shows an example calculation of the effective weights ($W_n = \frac{A_n \delta_{nX}}{\sum_a A_a - \sum_b A_b}$) to determine the species-aware order parameters, $Q_X^{order}$, shown in Eq. 9. For the example shown in Fig. 3(a), we obtain 3 paths connecting the order = 1 neighbors, each with weight $W_n = 1/4$. There are 7 paths each with weight $W_n = 1/4 \times 1/3$ connecting atom at '0' with order = 2 neighbors. And there are 19 paths for for order = 3 neighbors, each with weight $W_n = 1/4 \times 1/3 \times 1/3$. The resulting $W_n$'s are used to calculate the species-aware order parameters, $Q_X^{order}$. If a species-aware restriction is applied in the denominator, the resulting order parameter values become unbounded ($> 1$). And, their sum is system size dependent, adding up to $\sim N$, the total number of atoms in the system. Thus, we do not impose any restriction on the denominator, to keep the order parameter definitions unrelated to the system size.

To represent the anisotropy in the bonding environment of a superlattice uniquely, we define a species-aware, directionally-biased order parameter for atom $X$ as follows:

$$Q_X^{\Omega,order} = \sum_{paths} \prod_{steps}^{order} \frac{\overrightarrow{\omega_n} A_n \delta_{nX}}{\sum_a \overrightarrow{\omega_a} A_a - \sum_b \overrightarrow{\omega_b} A_b}. \tag{10}$$

The bias is implemented by considering only the projections of the face area $A_n$, that is being crossed by the step, along a chosen direction. We thus decompose the effective weights of each step along the graph into ($x$, $y$, $z$) components, and include only the specific component representing the chosen direction to calculate the order parameters. $\Omega(\overrightarrow{\omega})$ represents an imposed bias that allows contributions from a chosen direction, marked by the vector $\overrightarrow{\omega} = (\omega_x, \omega_y, \omega_z)$, where $\omega_x$, $\omega_y$, $\omega_z$ are the projections of $A_n$ onto the corresponding Cartesian directions, ($x$, $y$, $z$), respectively. The choice of $\overrightarrow{\omega}$ is not unique, any function of the interatomic distances could be chosen as the bias. The specific functional form of $\omega$ we chose is given by: $\omega_x = \cos^2\phi \sin^2\theta$, $\omega_y = \sin^2\phi \sin^2\theta$, $\omega_z = \cos^2\theta$, where $\theta$ and $\phi$ are the polar and azimuthal angles of the interatomic distance vector

(a)

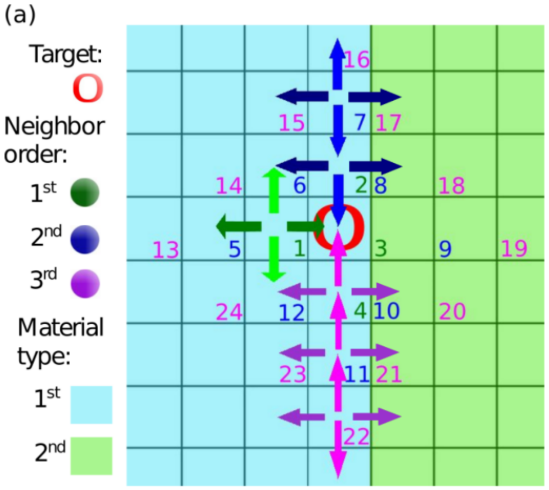


(b)

Order = 1

1→0 2→0 4→0

x direction:
$W_n$:
{½} {0} {0}
Total = 1/2

y direction:
$W_n$:
{0} {½} {½}
Total = 1

Order = 2

7→2→0 5→1→0 6→1→0
6→2→0 11→4→0 12→1→0
12→4→0

x direction:
$W_n$:
{0, 0} {½, 1} {0, 1}
{½, 0} {0, 0} {0, 1}
{½, 0}
Total = 1/2

y direction:
$W_n$:
{½, 1} {0, 0} {½, 0}
{0, 1} {½, 1} {½, 0}
{0, 1}
Total = 1

Order = 3

1→6→2→0 1→12→4→0 2→6→1→0
4→12→1→0 13→5→1→0 14→6→1→0
14→6→2→0 14→5→1→0 15→6→1→0
15→6→2→0 15→7→2→0 16→7→2→0
22→11→4→0 23→12→1→0 23→12→4→0
23→11→4→0 24→12→1→0 24→12→4→0
24→5→1→0

x direction:
$W_n$:
{0, 1, 0} {0, 1, 0} {½, 0, 1}
{½, 0, 1} {½, 1, 1} {½, 0, 1}
{½, 1, 0} {0, 1, 1} {0, 0, 1}
{0, 1, 0} {½, 0, 0} {0, 0, 0}
{0, 0, 1} {0, 0, 1} {0, 1, 0}
{½, 0, 0} {½, 0, 1} {½, 1, 0}
{0, 1, 1}
Total = 1/2

y direction:
$W_n$:
{½, 0, 1} {½, 0, 1} {0, 1, 0}
{0, 1, 0} {0, 0, 0} {0, 1, 0}
{0, 0, 1} {½, 0, 0} {½, 1, 0}
{½, 0, 1} {0, 1, 1} {½, 1, 1}
{½, 1, 0} {½, 1, 0} {½, 0, 1}
{0, 1, 1} {0, 1, 0} {0, 0, 1}
{½, 0, 0}
Total = 1/2

FIG. 4. (a) Example of a 2D graph of a square Voronoi lattice, including an interface between materials of types 1 and 2. The paths are constructed ending at the target atom 0, of material type 1. $\overrightarrow{\omega} = \{1, 0\}$ for the horizontal steps and $\overrightarrow{\omega} = \{0, 1\}$ for the vertical steps. (b) Effective weights for each path and the total directionally biased order parameter for atom 0.

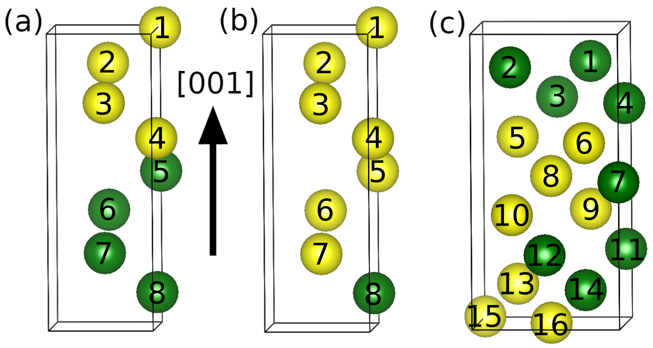


FIG. 5. Selected configurations to demonstrate the order parameter concept: (a) $Si_4Ge_4$ SL, (b) $Si_7Ge_1$ SL, (c) $Si_8Ge_8$ random alloy.

$\overrightarrow{d_n}$ makes with the Cartesian axes, as shown in Fig. 1. The functional form of $\overrightarrow{\omega}$ was selected because the sum of the components of $\overrightarrow{\omega}$ is equal to 1. For a specific choice of direction, $i = (x,\ y,\ z)$, the order parameter is given by

$$Q_X^{i,order} = \sum_{paths} \prod_{steps}^{order} \frac{\omega_{i,n} A_n \delta_{nX}}{\sum_a \omega_{i,a} A_a - \omega_{i,b} A_b}, \quad (11)$$

where

$$\begin{aligned} \overrightarrow{\omega}_m &= (\omega_{x,m},\ \omega_{y,m},\ \omega_{z,m}) \\ &= (\cos^2\phi_m \sin^2\theta_m,\ \sin^2\phi_m \sin^2\theta_m, \cos^2\theta_m) \quad (12) \end{aligned}$$

The order parameter feature $Q_X^{\Omega,order}$ is particularly important since directional ordering has been predicted to control the atomic orbital contributions to energy bands in Si/Ge heterostructures [6]. The bias in the denominator reflects the idea of conditional probability and results in values that are bounded $[0, 1]$. Without the bias, the order parameter values are not bounded.

The effective weights shown in Fig. 3 do not consider any imposed directional bias. If the directional bias is applied the weights would be considered separately for horizontal and vertical directions. We demonstrate the concept of the species-aware and directionally-biased order parameters in Fig. 4 using an illustrative example of a graph connecting atom at position '0' (representing $X$) with neighboring atoms, within a square Voronoi lattice including an interface between two materials. Only paths connecting atom 0 with other type 1 atoms are chosen, to determine species-aware order parameters. Green, blue, and purple arrows represent non-backtracking paths of lengths 1, 2, and 3, respectively. To represent the directionality of the paths, parallel or perpendicular to the interface, two different shades of the same color are used. Only non-backtracking steps are shown with the arrows. Figure 4(b) shows an example calculation of the effective weights ($W_n^i = \frac{\omega_{i,n} A_n \delta_{nX}}{\sum_a \omega_{i,a} A_a - \sum_b \omega_{i,b} A_b}$, $i = x,\ y$) to determine the species-aware and directionally-biased order parameters, $Q_X^{\Omega,order}$, shown in Eq. 10. For the example shown in Fig. 4(a), we obtain 3 paths connecting the order $= 1$ neighbors to atom '0', each with effective weight $W_n^i = 1/2$. The directional aspect is reflected by the fact that only $W_n^x \neq 0$ for the path $1 \to 0$ and $W_n^y \neq 0$ for the paths $2 \to 0$ and $4 \to 0$. There are 7 paths connecting order $= 2$ neighbors with atom at '0' with only non-zero weights $W_n^x = 1/2 \times 1$ for the $5 \to 1 \to 0$ path and $W_n^y = 1/2 \times 1$ for the $7 \to 2 \to 0$ and $11 \to 4 \to 0$ paths. There are 19 paths for order $= 3$ neighbors, with only non-zero weights $W_n^x = 1/2 \times 1 \times 1$ for $13 \to 5 \to 1 \to 0$ and $W_n^y = 1/2 \times 1 \times 1$ for $16 \to 7 \to 2 \to 0$. The resulting $W_n^i$'s are used to calculate the order parameters, $Q_X^{x,order}$ and $Q_X^{y,order}$. If $W_n$ is 1/2 then we have 50% chance of a step to be towards the target. $W_n$ is 1 if once subtract the backtracking step, so we have 100% chance to step towards the target. This is where the conditional probability plays role. If this would be non-conditional, then we would have 1/4 and 1/3 (as shown in Fig. 2) instead of 1/2 and 1.

TABLE I. $Si_4Ge_4$ SL order parameters

| Atom | # | $Q^{x,1}$ | $Q^{y,1}$ | $Q^{z,1}$ | $Q^{x,2}$ | $Q^{y,2}$ | $Q^{z,2}$ | $Q^{x,3}$ | $Q^{y,3}$ | $Q^{z,3}$ |
|---|---|---|---|---|---|---|---|---|---|---|
| Si | 1 | 0.55 | 0.55 | 0.51 | 0.49 | 0.49 | 0.45 | 0.36 | 0.36 | 0.29 |
| Si | 2 | 0.95 | 0.95 | 0.89 | 0.64 | 0.64 | 0.53 | 0.43 | 0.43 | 0.34 |
| Si | 3 | 0.95 | 0.95 | 0.89 | 0.64 | 0.64 | 0.53 | 0.43 | 0.43 | 0.34 |
| Si | 4 | 0.55 | 0.55 | 0.51 | 0.49 | 0.49 | 0.45 | 0.36 | 0.36 | 0.29 |
| Ge | 5 | 0.53 | 0.53 | 0.49 | 0.47 | 0.47 | 0.46 | 0.37 | 0.37 | 0.30 |
| Ge | 6 | 0.97 | 0.97 | 0.94 | 0.70 | 0.70 | 0.58 | 0.47 | 0.47 | 0.36 |
| Ge | 7 | 0.97 | 0.97 | 0.94 | 0.70 | 0.70 | 0.58 | 0.47 | 0.47 | 0.36 |
| Ge | 8 | 0.53 | 0.53 | 0.49 | 0.47 | 0.47 | 0.46 | 0.37 | 0.37 | 0.30 |

In Table I, we show the calculated species aware and directionally biased order parameters for the $Si_4Ge_4$ SL configuration shown in Fig. 5(a). The corresponding atom numbers (column 2) are shown as labels in Fig. 5(a). We note that the order parameter values are higher for the inner atoms and lower for the interface atoms. This is due to the presence of greater number of same species neighboring atoms for the inner atoms, resulting in higher number of connecting paths contributing to the order parameters. For comparison, all the listed order parameters are equal to 1 for the bulk systems. The order parameters in the $x$ and the $y$ directions are equal, due to the symmetry of the configuration. The order parameter values decrease for higher order neighbors, as expected. Ordering in the $z$ direction is lower and decreases faster with the order number than the ordering in the $x$ and $y$ directions. This reflects the orientation of the heterogeneous stacking along the $z$ direction.

The calculated order parameters for the $Si_7Ge_1$ SL depicted in Fig. 5(b) are shown in Table II. Similar observations can be made that the ordering is higher for the inner atoms and lower for the interface atoms. The order parameter values are particularly low for the *Ge* atom since

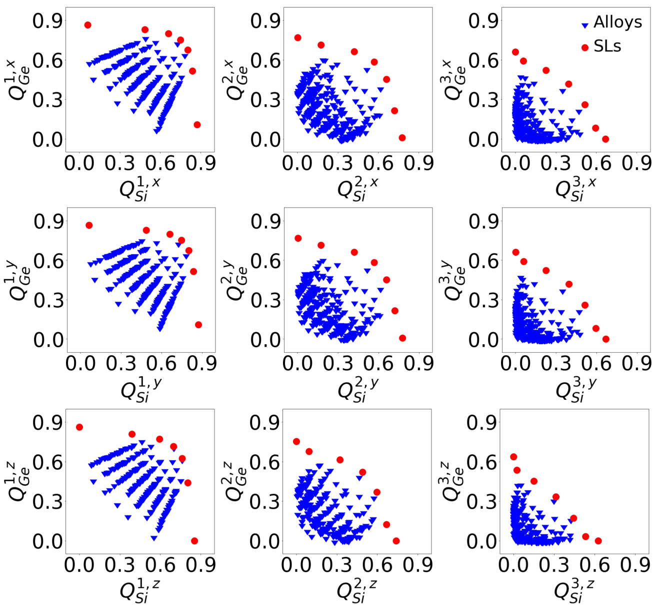


FIG. 6. Directionally biased order parameters.

TABLE II. $Si_7Ge_1$ SL order parameters

| Atom | # | $Q^{x,1}$ | $Q^{y,1}$ | $Q^{z,1}$ | $Q^{x,2}$ | $Q^{y,2}$ | $Q^{z,2}$ | $Q^{x,3}$ | $Q^{y,3}$ | $Q^{z,3}$ |
|---|---|---|---|---|---|---|---|---|---|---|
| Si | 1 | 0.60 | 0.60 | 0.58 | 0.53 | 0.53 | 0.52 | 0.45 | 0.45 | 0.43 |
| Si | 2 | 0.96 | 0.96 | 0.90 | 0.73 | 0.73 | 0.67 | 0.65 | 0.65 | 0.60 |
| Si | 3 | 1.00 | 1.00 | 1.00 | 0.96 | 0.96 | 0.91 | 0.80 | 0.80 | 0.74 |
| Si | 4 | 1.00 | 1.00 | 1.00 | 0.99 | 0.99 | 0.98 | 0.90 | 0.90 | 0.82 |
| Si | 5 | 1.00 | 1.00 | 1.00 | 0.96 | 0.96 | 0.91 | 0.80 | 0.80 | 0.74 |
| Si | 6 | 0.96 | 0.96 | 0.90 | 0.73 | 0.73 | 0.67 | 0.65 | 0.65 | 0.60 |
| Si | 7 | 0.60 | 0.60 | 0.58 | 0.53 | 0.53 | 0.52 | 0.45 | 0.45 | 0.43 |
| Ge | 8 | 0.11 | 0.11 | 0.00 | 0.01 | 0.01 | 0.00 | 0.00 | 0.00 | 0.00 |

the $Ge$ region is only 1 monolayer thick. The thinner the layer the smaller the $Q^{z,order}$, due to the reduced number of same-species neighbors and as a result, availability of fewer connecting paths. We can identify four unique atomic environments along the $z$ direction: interface Si, interface Ge, inner Si, and inner Ge. For example, considering Fig. 5 and Tables I and II, we can classify that the interface atoms are characterized by $Q^{z,1} \sim 0.5-0.6$ and the inner atoms have $Q^{z,1} \sim 0.9-1.0$. The size of these regions distinguishes different configurations. For example, in the $Si_4Ge_4$ configuration, we can identify the following regions: interface Si (1,4); inner Si (2,3); interface Ge (5,8); inner Ge (6,7). As expected, the boundaries between different regions become more clear with the increase of the systems size.

In Table III, we show the calculated species aware and directionally biased order parameters for the $Si_8Ge_8$ random alloy configuration shown in Fig. 5(c). Unlike the SL configurations, the order parameters do not show any specific pattern and decrease fast with the order number reflecting the disordered nature of the system. In Fig. 6, we show the directionally biased order parameters of all the random alloy and strain-symmetrized SL unit configurations in the training set.

TABLE III. $Si_8Ge_8$ random alloy order parameters

| Atom | # | $Q^{x,1}$ | $Q^{y,1}$ | $Q^{z,1}$ | $Q^{x,2}$ | $Q^{y,2}$ | $Q^{z,2}$ | $Q^{x,3}$ | $Q^{y,3}$ | $Q^{z,3}$ |
|---|---|---|---|---|---|---|---|---|---|---|
| Ge | 1 | 0.50 | 0.55 | 0.48 | 0.21 | 0.21 | 0.15 | 0.09 | 0.08 | 0.05 |
| Ge | 2 | 0.55 | 0.50 | 0.48 | 0.23 | 0.21 | 0.17 | 0.08 | 0.08 | 0.04 |
| Ge | 3 | 0.55 | 0.50 | 0.48 | 0.21 | 0.21 | 0.15 | 0.08 | 0.09 | 0.05 |
| Ge | 4 | 0.50 | 0.55 | 0.48 | 0.21 | 0.23 | 0.17 | 0.08 | 0.08 | 0.04 |
| Si | 5 | 0.34 | 0.34 | 0.30 | 0.22 | 0.22 | 0.20 | 0.05 | 0.05 | 0.04 |
| Si | 6 | 0.34 | 0.34 | 0.30 | 0.21 | 0.21 | 0.20 | 0.05 | 0.05 | 0.04 |
| Ge | 7 | 0.10 | 0.10 | 0.19 | 0.05 | 0.05 | 0.08 | 0.02 | 0.02 | 0.03 |
| Si | 8 | 0.83 | 0.83 | 0.83 | 0.11 | 0.11 | 0.09 | 0.03 | 0.03 | 0.03 |
| Si | 9 | 0.34 | 0.37 | 0.34 | 0.22 | 0.23 | 0.22 | 0.05 | 0.05 | 0.03 |
| Si | 10 | 0.37 | 0.34 | 0.34 | 0.23 | 0.22 | 0.22 | 0.05 | 0.05 | 0.03 |
| Ge | 11 | 0.34 | 0.29 | 0.26 | 0.09 | 0.10 | 0.08 | 0.02 | 0.02 | 0.02 |
| Ge | 12 | 0.29 | 0.34 | 0.26 | 0.10 | 0.09 | 0.08 | 0.02 | 0.02 | 0.02 |
| Si | 13 | 0.45 | 0.45 | 0.49 | 0.05 | 0.05 | 0.03 | 0.02 | 0.02 | 0.02 |
| Ge | 14 | 0.46 | 0.46 | 0.51 | 0.08 | 0.08 | 0.08 | 0.03 | 0.03 | 0.02 |
| Si | 15 | 0.30 | 0.30 | 0.21 | 0.09 | 0.09 | 0.07 | 0.01 | 0.01 | 0.01 |
| Si | 16 | 0.30 | 0.30 | 0.21 | 0.09 | 0.09 | 0.07 | 0.01 | 0.01 | 0.01 |

We compute the mean, mean absolute deviation, maximum, and minimum of the order parameter distributions in a configuration to create the ordering features. In total, our method describes each configuration by 36 order parameter features: (3 orders)×(3 directional bias)×(4 statistical features).

**Feature Importance**

In Fig. 7 and 8, we show the relative importance of 35 features of the ideal substrate strained SiGe SL training configurations and random alloy SiGe and strain-symmetrized SL configurations,respectively, that have the most impact on the outcomes of the RF algorithms. The total importance factors of all 100 features is 1. We notice that the features derived from the crystal graph play an important role for both the systems. The order parameters become more important for the random alloys than in the case of strained ideal SLs. For the alloys, the first order parameter $Q^{y,1}_{X}$ is at the sixth place among 100 total features. Considering the trend, we anticipate that the order parameter features would become more important for the electronic properties of complex structures that include a combination of alloy and heterogeneous regions or large random alloy configurations.

## SEEBECK CALCULATION

We checked the convergence of the calculated thermopower of representative $Si_{16}Ge_{16}$ random alloy with respect to three main parameters: number of $k$-points, number of bands, and electronic band gap. The effect

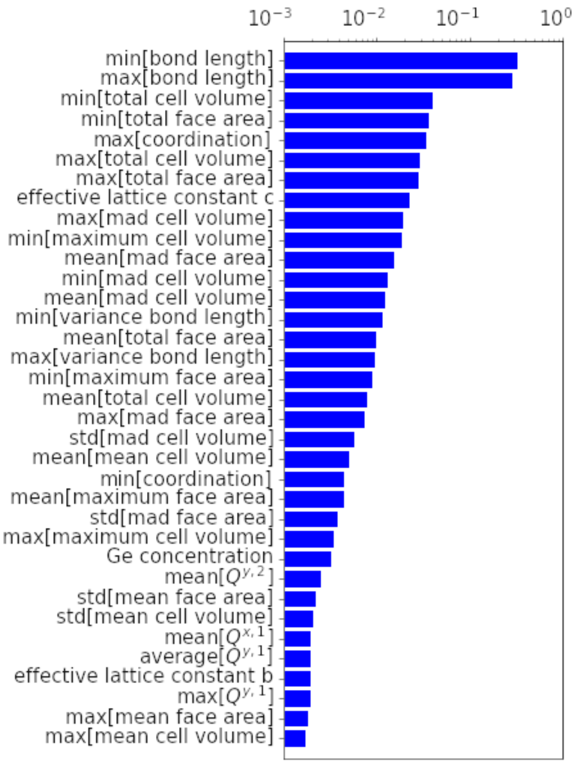


FIG. 7. The top 35 most importance features of the training structures, that control the predictions of the random forests algorithm: the dominant features of the strained ideal superlattice configurations.

of increasing $k$-point mesh on the thermopower without and with band gap correction is shown in Fig. 9(a) and Fig. 9(b), respectively. The results with $21 \times 21 \times 21$ k-point mesh are indistinguishable from a denser $31 \times 31 \times 31$ mesh, therefore we chose a $\Gamma$-centered $21 \times 21 \times 21$ Monkhorst-Pack $k$-point mesh for the production calculations shown in the main manuscript. The band gap correction affects thermopower values at low ($n_e \sim 10^{17}$) carrier concentrations, the contribution from the valence band maximum increases the thermopower, and but is not significant for the higher concentrations. In Fig. 10 we demonstrate the convergence of $S$ by including increasing number of conduction bands in the calculation. For the main results of the manuscript, we trained the ML algorithms on 6 conduction and 6 valence bands and included the 12 bands to compute the Seebeck coefficients.

## NON-IDEAL HETEROSTRUCTURES

We tested the ML models on a class of non-ideal heterostructures including the structures shown in Fig. 5 in the main manuscript. We constructed the test configurations by stacking the SL unit cells with atomic

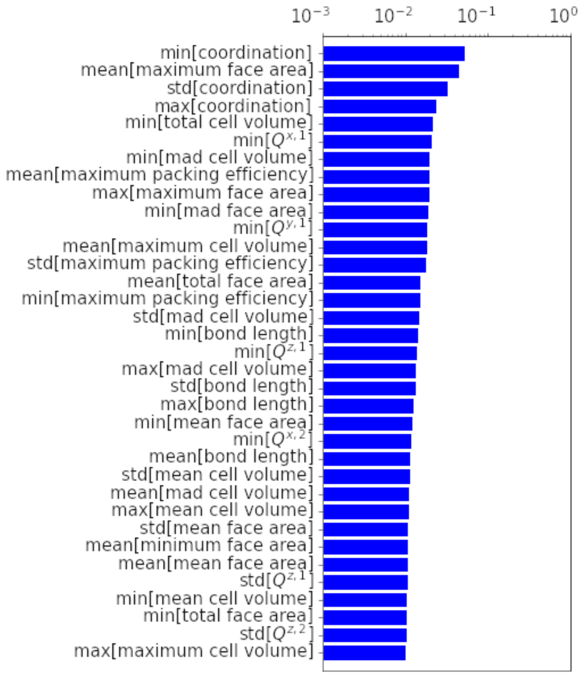


FIG. 8. The top 35 most importance features of the training structures, that control the predictions of the random forests algorithm: the dominant features of the random alloy configurations and strain-symmetrized SL configurations.

composition $Si_nGe_m$ (16 atoms, 2 CCs) along the [001] (Fig. 11(b)) and [100] (Fig. 11(a)) directions, and with uneven repeat units. The resulting stoichiometry of the test configurations can be represented as $Si_nGe_mSi_kGe_l$ with $n+m+k+l = 32$, $n \neq k$, and $m \neq l$. We tested our ML models on all the $2\times C^4_2$ generated test structures and show only some results representing the systems, for the sake of brevity. Figure 11 shows the predicted and DFT obtained thermopower two strain-symmetrized non-ideal heterostructures.

## SCRIPTS AND DATASETS

We have made the Python scripts available for extracting the geometrical features from an example data set [7]. The example data set includes 49 Si/Ge superlattice (SL) configurations with external substrate induced strain. We have included the SL geometry data before and after DFT relaxation, and the DFT calculated energy values.

* sanghamitra.neogi@colorado.edu

[1] L. Ward, R. Liu, A. Krishna, V. I. Hegde, A. Agrawal, A. Choudhary, and C. Wolverton, Including crystal structure attributes in machine learning models of formation

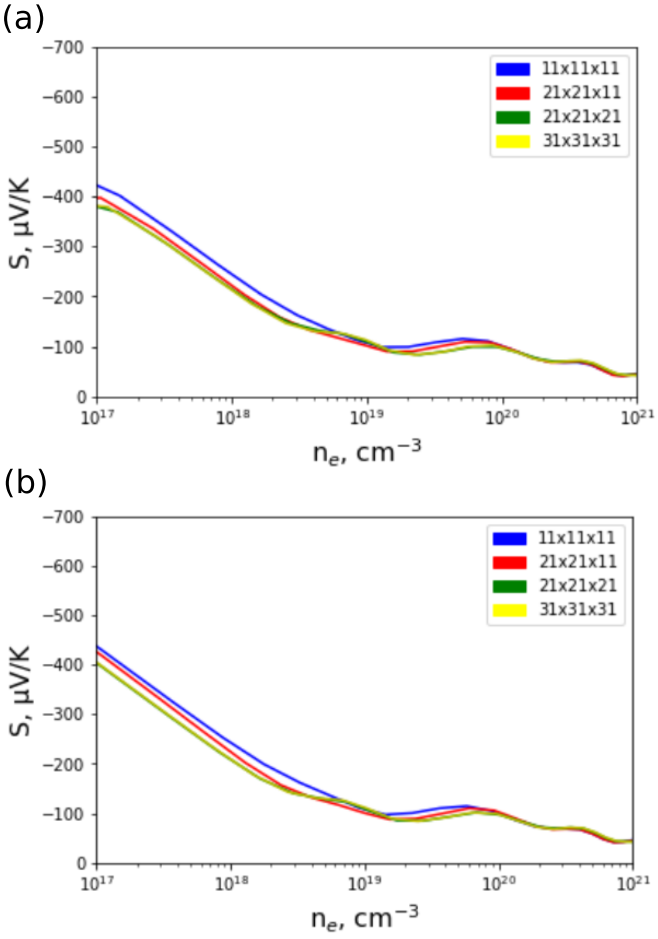


FIG. 9. Thermopower convergence for $Si_{16}Ge_{16}$ strain-symmetrized random alloy with increasing the $k$-point mesh. We chose a Γ-centered $21 \times 21 \times 21$ Monkhorst-Pack $k$-point mesh for the production calculations. (a) and (b) show the convergence of $S$ without and with band gap corrections, respectively, establishing the robustness of transport property results irrespective of band gap values.

energies via voronoi tessellations, Physical Review B **96**, 024104 (2017).

[2] J. Cowley, An approximate theory of order in alloys, Physical Review **77**, 669 (1950).

[3] T. Xie and J. C. Grossman, Crystal graph convolutional neural networks for an accurate and interpretable prediction of material properties, Physical review letters **120**, 145301 (2018).

[4] T. Xie and J. C. Grossman, Hierarchical visualization of materials space with graph convolutional neural networks, The Journal of chemical physics **149**, 174111 (2018).

[5] S. Gong, T. Xie, T. Zhu, S. Wang, E. R. Fadel, Y. Li, and J. C. Grossman, Predicting charge density distribution of materials using a local-environment-based graph convolutional network, Physical Review B **100**, 184103 (2019).

[6] V. Proshchenko, M. Settipalli, A. K. Pimachev, S. Neogi, *et al.*, Modulation of semiconductor superlattice thermopower through symmetry and strain, arXiv preprint arXiv:1907.03461 (2019).

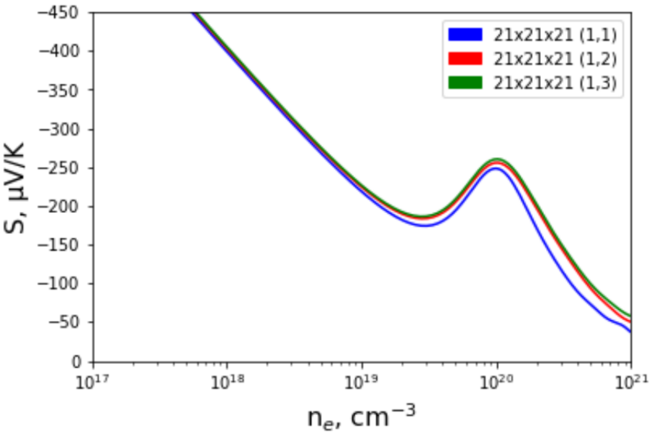


FIG. 10. Thermopower convergence for $Si_8Ge_8$ strain-symmetrized SL with increasing the number of conduction bands in the calculation. The number of included conduction bands is varied from 1 to 3 while keeping the number of valence bands fixed to one. In the results presented in the main manuscript we train the ML algorithms to learn 6 conduction and 6 valence bands and include them to compute the Seebeck coefficients.

[7] Cuantam lab - github page, `https://github.com/CUANTAM`.

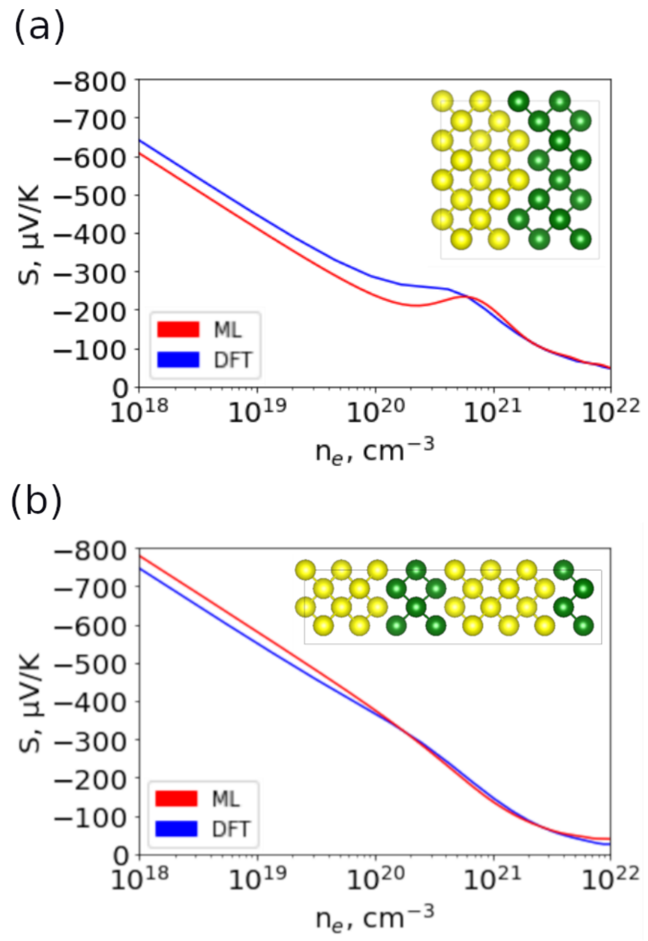


FIG. 11. Predicted and DFT computed thermopower of (a) $Si_{32}Ge_{32}$ strain-symmetrized non-ideal heterostructure and (b) strain-symmetrized $Si_5Ge_3Si_6Ge_2$ multilayered structure. The prediction is made with RF algorithm trained on random alloy and strain-symmetrized unit structures.
